# Supplementary material for: Elastoplasticity Mediates Dynamical Heterogeneity Below the Mode-Coupling Temperature
Source: arXiv:2103.01852 ancillary file (2021-03-05)
Supplement: Supplementary file 1 [file SM.pdf]

# Supplementary Material for "Elastoplasticity Mediates Dynamical Heterogeneity Below the Mode-Coupling Temperature"

Rahul N. Chacko,[1,2] François P. Landes,[3] Giulio Biroli,[4] Olivier Dauchot,[5] Andrea J. Liu,[1] and David R. Reichman[6]
[1]*Department of Physics and Astronomy, University of Pennsylvania, Philadelphia, Pennsylvania 19104, USA*
[2]*Department of Physics and James Franck and Enrico Fermi Institutes, University of Chicago, Chicago, Illinois 60637, USA*
[3]*Université Paris-Saclay, CNRS, Laboratoire Interdisciplinaire des Sciences du Numérique, 91400, Orsay, France*
[4]*Laboratoire de Physique de l'école normale supérieure, ENS, Université PSL, CNRS, Sorbonne Université, Université Paris-Diderot, Sorbonne Paris Cité, 75005 Paris, France*
[5]*UMR Gulliver 7083 CNRS, ESPCI ParisTech, PSL Research University, 10 rue Vauquelin, 75005 Paris, France*
[6]*Department of Chemistry, Columbia University, 3000 Broadway, New York, New York 10027, USA*
(Dated: March 4, 2021)

## I. LENGTH SCALES AND TIME SCALES

### A. Dynamical heterogeneity length scale and Mermin-Wagner fluctuations

We mitigate the effects of Mermin-Wagner fluctuations on our two-dimensional system [1–3] by subtracting from the displacement of each particle $i$ that of the center-of-mass of particles $j$ with centers within some distance $R_{\mathrm{MW}}$ of particle $i$ [2, 3]:

$$\Delta \boldsymbol{r}_i(t,t') = \boldsymbol{r}_i(t') - \boldsymbol{r}_i(t) - \langle \boldsymbol{r}_j(t') - \boldsymbol{r}_j(t)\rangle_j \,, \tag{1}$$

with $\langle\cdot\rangle_j$ the average calculated over $j \in \{|\boldsymbol{r}_j(t) - \boldsymbol{r}_i(t)| < R_{\mathrm{MW}}\} \cup \{|\boldsymbol{r}_j(t') - \boldsymbol{r}_i(t')| < R_{\mathrm{MW}}\}$. The union here is taken so as to preserve the antisymmetry of particle displacements under time reversal (see §II A). Following the literature, we will refer to this reduced displacement as the cage-relative displacement. A judicious choice of $R_{\mathrm{MW}}$ is needed to mitigate Mermin-Wagner fluctuations while preserving short-scale physics. Das *et al.* [4] have argued that the dynamical heterogeneity length scale $\xi_{\mathrm{dyn}}$ should be used. This can be obtained from the four-point structure function[5, 6]

$$S_4\left(\boldsymbol{k},t,t'\right) = N \mathrm{Var}\left[\hat{Q}\left(\boldsymbol{k},t,t'\right)\right] \tag{2}$$

at $t' = t + \tau_\alpha$, where the variance is calculated over ensembles, $N$ is the number of particles, and $\hat{Q}$ is the Fourier transform of the Gaussian overlap function. We have

$$\hat{Q}\left(\boldsymbol{k},t,t'\right) = \frac{1}{N}\sum_{i=1}^{N} e^{\mathrm{i}\boldsymbol{k}\cdot\boldsymbol{r}_i(0)} e^{-\left|\Delta \boldsymbol{r}_i(t,t')\right|^2/2a^2}, \tag{3}$$

where $\boldsymbol{r}_i\left(t\right)$ is the position of particle $i$ at time $t$ and $a$ is the plateau height of the root mean squared displacement (RMSD) (see §I C) of particles of the same species as particle $i$, a measure of the size of the cage formed by particles neighboring $i$. In practice, we fix $t = 0$. We take $\boldsymbol{k} = (k, 0)$ without loss of generality, and calculate the variance in Eq. 2 over 101 trajectories with independent initial equilibrium conditions per temperature.

The choice of $R_{\mathrm{MW}}$ used when calculating cage-relative displacements affects the plateau height $a$, the $\tau_\alpha$ time scale, and the calculation of $\hat{Q}$ itself, so we need to find a self-consistent choice of $R_{\mathrm{MW}}$ that leads to a value $\xi_{\mathrm{dyn}} = R_{\mathrm{MW}}$. To this end, we calculate $\tau_\alpha$ (Fig. 1(b)) and $a$ (not shown) as a function of $R_{\mathrm{MW}}$. For $a$, we calculate this for particles within ten log-spaced diameter bins (see Fig. 3) from the height of the RMSD at $\Delta t = 10$. To obtain $\tau_\alpha$, defined such that the self-intermediate scattering function

$$F\left(\boldsymbol{k},t,t'\right) = \frac{1}{N}\sum_{i=1}^{N} e^{\mathrm{i}\boldsymbol{k}\cdot\Delta\boldsymbol{r}_i(t,t')} \tag{4}$$

satisfies $F\left(k,t,t+\tau_\alpha\right)\big|_{k=2\pi} = 1/e$, we use the secant root-finding method on trajectory data averaged over 101 trajectories started from independent initial equilibrium configurations. We choose the wavenumber $k = 2\pi$, since the

wavelength $\lambda = 1$ corresponds to the radius of the first nearest neighbor shell of particles (§I B), so that $F(k) = 1/e$ corresponds to decorrelation between the positions of particles and the cage formed by nearest neighbors.

The result is plotted in Fig. 1(b). Having obtained $a$ and $\tau_\alpha$ corresponding to each $R_{\text{MW}}$ value and each temperature, we calculate $S_4(k, \tau_\alpha)$ following Lačević *et al.* [5, 6]. We extract a dynamic length scale $\xi$ from $S_4$ using an Ornstein-Zernike fit of $1/\left(1+\xi^2 k^2\right)$ to $S_4(k,\tau_\alpha)/S_4(k,0)$ for $k$ in some early regime (we choose $k \in [0, 1.5]$). Calculating this $\xi$ for each $R_{\text{MW}}$ value, we take $\xi_{\text{dyn}}$ to be the value of $\xi$ which most closely matches the input $R_{\text{MW}}$ value, as plotted in Fig. 1(a).

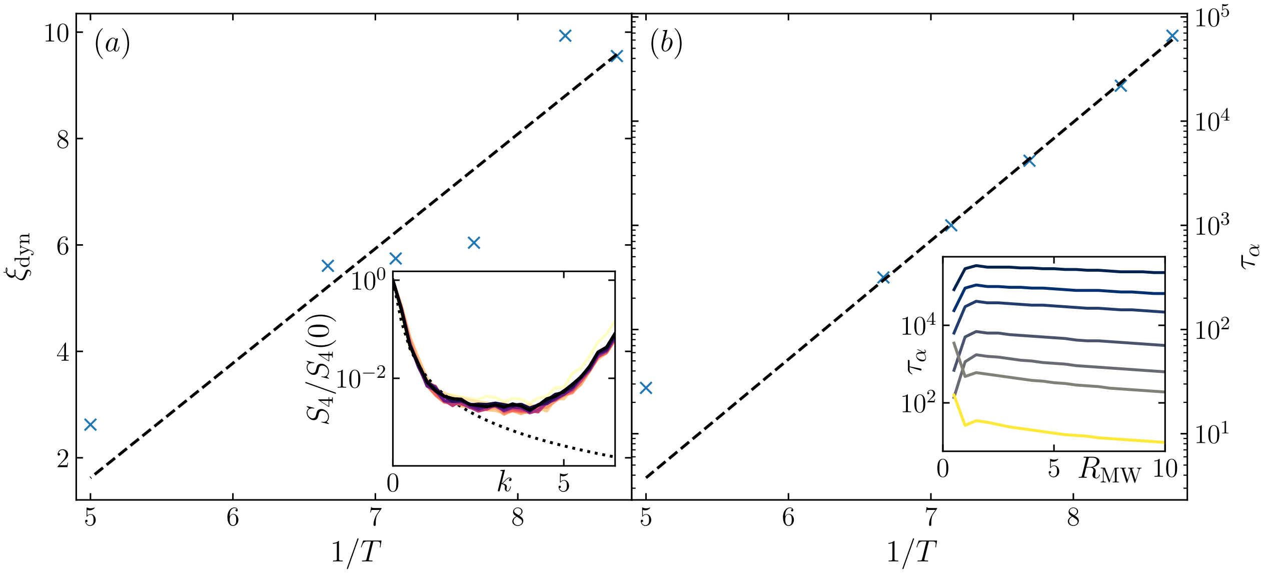


FIG. 1. *Self-consistent $R_{\text{MW}}$ selection procedure.* Main: (a) Dynamic length scale $\xi_{\text{dyn}}$, calculated with a self-consistent Mermin-Wagner coarse-graining length $R_{\text{MW}} = \xi_{\text{dyn}}$, and (b) the corresponding $\tau_\alpha$ time scale for that $R_{\text{MW}}$ value, plotted as a function of $1/T$. Dashed lines: linear fits to (a) $\xi_{\text{dyn}}$ under the constraint $\xi_{\text{dyn}}(T_{\text{onset}}) = 0$, $\xi_{\text{dyn}} = 2.15\,(1/T - 1/T_{\text{onset}})$, and (b) $\log \tau_\alpha$ for $T \geq 0.15$, $\tau_\alpha = 7.72 \times 10^{-6} \exp(2.62/T)$. Inset to (a): Plots of the normalized four-point structure factor for time interval $\tau_\alpha$, $S_4(k,\tau_\alpha)/S_4(0,\tau_\alpha)$, for a system at temperature $T = 0.115$ at $R_{\text{MW}} = 0.5, 1, 1.5, \ldots, 10$ (lighter to darker). The value of $\tau_\alpha$ is adjusted for each $R_{\text{MW}}$ value based on the inset to (b). The dashed line is an example Ornstein-Zernike fit to the region $k \in [0, 1.5]$. Inset to (b): $\tau_\alpha$ as a function of $R_{\text{MW}}$ for temperatures $T = 0.115$, 0.12, 0.13, 0.14, 0.15, 0.2 and 0.3 (darker to lighter).

Many quantities are quite insensitive to the value of $R_{\text{MW}}$, so long as it contains the first neighbor shell. This results in the wide spread of obtained $\xi_{\text{dyn}}$ values when plotted against $1/T$ seen in Fig. 1. To mitigate this, and to allow us to find $\xi_{\text{dyn}}$ for temperatures $T < 0.115$ for which we do not have trajectory data up to time $\tau_\alpha$, we fit a linear trend through the data, with $x$-intercept fixed such that $\xi_{\text{dyn}}(T_{\text{onset}}) = 0$. This linear trend can be justified from the linear trend seen for the point-to-set length $\xi_{\text{PTS}}$ [7], and the fact, observed in [4], that in two dimensions, $\xi_{\text{dyn}}$ and $\xi_{\text{PTS}}$ scale similarly to one another. Similarly, an exponential growth for $\tau_\alpha$ as a function of $1/T$ for low values of $T$ is consistent with what was seen in [7], and allows us to estimate the value of $\tau_\alpha$ for temperatures below $T = 0.115$.

To summarize, we set $R_{\text{MW}} = \xi_{\text{dyn}} = \min\{0, 2.15\,(1/T - 1/T_{\text{onset}})\}$ and, for the temperature range $T \geq 0.15$ considered in this report, $\tau_\alpha = 7.72 \times 10^{-6} \exp(2.62/T)$.

### B. First-neighbor shell size

We plot, in Fig. 2, the pair distribution

$$g(\boldsymbol{r}, t) := \frac{V}{N} \left\langle \sum_{j \neq i} \delta\left(\boldsymbol{r} - \boldsymbol{r}_{ij}(t)\right) \right\rangle_i \tag{5}$$

of our system, where $i, j \in \{1, 2, \ldots, N\}$ label particles, $\boldsymbol{r}_i$ is the position of particle $i$ at time $t$, $\boldsymbol{r}_{ij} := \boldsymbol{r}_j - \boldsymbol{r}_i$ is the separation vector between particles $i$ and $j$, $V = L^2$ is the area of the system, and $\langle \cdot \rangle_i$ is the average is over all

particles $i$ in the system. More precisely, we plot $g(r) := \langle g(\boldsymbol{r}, 0)\rangle_{|\boldsymbol{r}|=r}$, since our system is isotropic and stationary, and average this over 202 configurations per temperature. We see, in particular, that the first neighbour shell occurs at separation $r \approx 1$, corresponding to the mean particle diameter. We note that the local environment of particles varies considerably as a function of particle diameter (Fig. 2, inset).

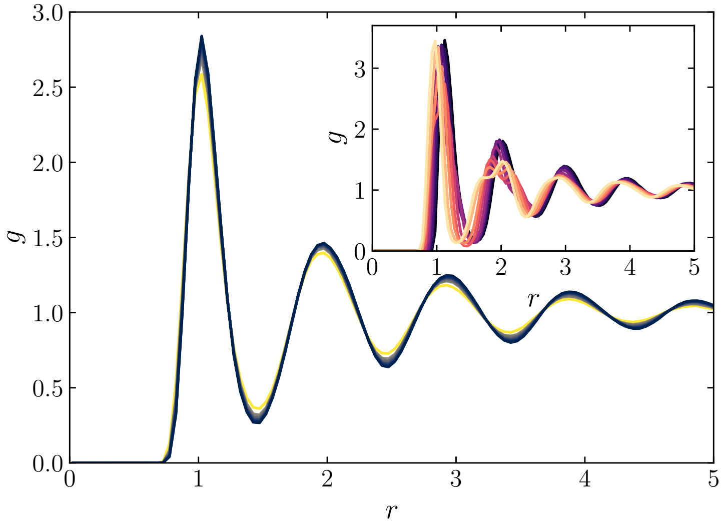


FIG. 2. *Particle-dependent shell sizes.* Pair distribution $g(r)$ for temperatures $T = 0.1$, 0.105, 0.11, 0.115, 0.12, 0.13, 0.14, 0.15, and 0.2 (curves darker to lighter). Inset: $g$ for particles separated into ten bins of particle diameter (darker color denoting larger diameter) with bin edges logarithmically spaced in the interval $[\sigma_{\min}, \sigma_{\max}]$ at temperature $T = 0.1$.

### C. Plateau start time and height

We plot the root mean squared displacement

$$\mathrm{RMSD}(t, t') := \sqrt{\left\langle |\Delta\boldsymbol{r}_i(t, t')|^2 \right\rangle_i} \tag{6}$$

in Fig. 3. Here, $\Delta\boldsymbol{r}_i(t, t')$ is the cage-relative (see §I A) displacement of particle $i$ between times $t$ and $t'$. As above, steady state means that in practice we plot $\mathrm{RMSD}(\Delta t) = \mathrm{RMSD}(0, \Delta t)$, and average over 101 equilibrium trajectories. We see that for the range of temperatures we consider in this study, the RMSD plateau starts at around $\Delta t = 2$, with $\mathrm{RMSD}(\Delta t = 10)$ providing a reasonable choice of plateau height definition. There is a noticeable diameter-dependence of the RMSD plateau height, as can be seen in the inset to Fig. 3.

### D. Rearrangement duration and amplitude criterion

We wish to identify a rearrangement time scale $\Delta t$ for individual rearrangements. We use a slight variation of a strategy introduced by Cubuk *et al.* [8]. The idea is that displacements in excess of the average inside-cage motion are correlated over short distances and over a relatively short time scale. This short time scale may be thought of as the clustering time: it corresponds to a couple of single-particle events following each other closely in space and time. Here we identify this time scale $\Delta t$ and adopt it as the size of the time intervals across which we study rearrangements. Letting $a_i$ be the RMSD plateau height (see previous subsection) for particles within the same diameter bin as particle $i$ and

$$\Delta_i(\Delta t) := \frac{|\Delta\boldsymbol{r}_i(0, \Delta t)|^2}{a^2}, \tag{7}$$

we calculate the normalized spatial correlation function of the motion of particles at a distance $\boldsymbol{r}$:

$$\mathrm{Corr}(\boldsymbol{r}, \Delta t) := \frac{\left\langle \sum_{j\neq i} \Delta_i \Delta_j \delta\big(\boldsymbol{r} - \boldsymbol{r}_{ij}(0)\big) \right\rangle_i - \langle \Delta_i \rangle_i^2}{\mathrm{Var}_i[\Delta_i]}, \tag{8}$$

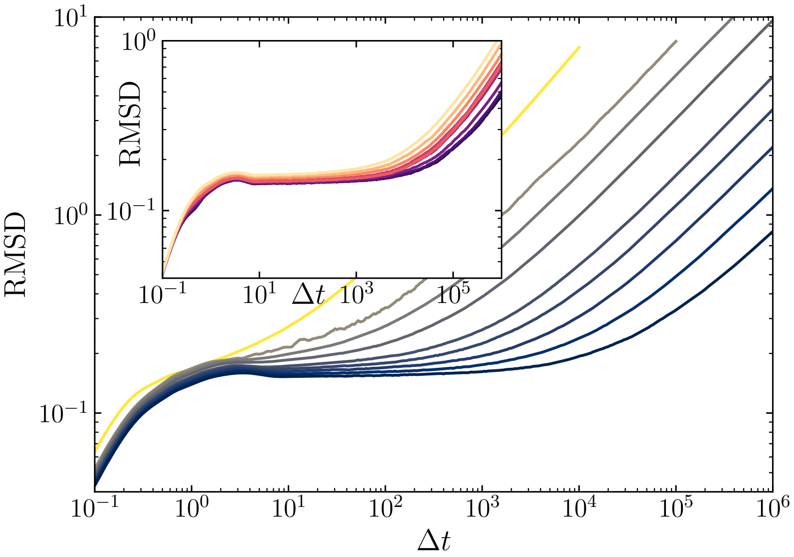


FIG. 3. *Estimation of the cage size $a$.* Root mean squared displacement RMSD for temperatures $T = 0.1$, 0.105, 0.11, 0.115, 0.12, 0.13, 0.14, 0.15, and 0.2 (curves darker to lighter). Inset: RMSD for particles separated into ten bins of particle diameter (darker color denoting larger diameter) with log-spaced bin edges at temperature $T = 0.1$.

where we omit the argument $\Delta t$ in $\Delta_i\left(\Delta t\right)$ for notational convenience, where $\mathrm{Var}_i\left[\cdot\right]$ denotes the variance over particles $i$. As in previous sections, we note that $\mathrm{Corr}\left(\boldsymbol{r}, \Delta t\right) = \mathrm{Corr}\left(r, \Delta t\right)$, and so average over $\{|\boldsymbol{r}| = r\}$ when plotting Corr in the inset to Fig. 4. As seen in this inset, Corr decays exponentially as a function of $\Delta r$, allowing us to identify a decay length $\xi_{\mathrm{c}}$ as a function of time interval length $\Delta t$.

We plot this in the Fig. 4(a) for temperatures $T = 0.1$, 0.105, 0.11, 0.115, 0.12, 0.13, 0.14 and 0.15. We see that all our temperatures have a minimum roughly in the interval $\Delta t \in [10^1, 10^2]$. At the smallest $\Delta t$, we are merely correlating ballistic trajectories of particles, or, near $10^0$, the rattling of particles within cages. At larger $\Delta t$, some cage-breaking events are able to occur, and the correlation length decreases as a result. At yet larger $\Delta t$, rearrangements have time to trigger nearby rearrangements, and $\xi_{\mathrm{c}}$ is seen to grow again. A $\Delta t$ which minimizes $\xi_{\mathrm{c}}$ should therefore correspond roughly to the single-rearrangement time scale we desire. We choose $\Delta t = 10^2$ for our rearrangement time scale, since it is in the minimising plateau for all temperatures under consideration, while also being well above the ballistic time scale.

We choose our criterion $\Delta_i > 5$ for what constitutes a rearrangement from the good qualitative match this produces between the overall displacement of the system in time $\tau_\alpha$ and the locations of individual hops across the rearrangement time $\Delta t$, as shown for $T = 0.12$ in Figs. 4(b-c). Getting such a correspondence involves choosing a threshold large enough that transient, reversible rearrangements are filtered out, and small enough that the incremental rearrangements across time $\Delta t$ that build up the overall displacement field across time $\tau_\alpha$ are picked up.

As seen in Fig. 4(a), the minimum of the rearrangement correlation length $\xi_{\mathrm{c}}$ is flat across a number of decades at low temperatures. Alternative choices of rearrangement time scale $\Delta t$ might also seem justified. For instance, a rearrangement time $\Delta = 10^1$, corresponding to the beginning of the low-$\xi_{\mathrm{c}}$ plateau in Fig. 4(a), would be closer to the minimum for our highest temperature $T = 0.15$, at the cost of being closer to the ballistic time scale.

We have checked (Fig. 5) that the key result of our manuscript, namely the drastic increase in long-range mean squared anisotropy $\alpha(r)$ in the pair distribution of rearrangements $g_{\mathrm{hop}}$ (see main text), is preserved if we adopt $\Delta t = 10^1$ instead of $\Delta t = 10^2$. This suggests that our results are robust to choices of $\Delta t$, at least within the low-$\xi_{\mathrm{c}}$ plateau.

### E. Strain cutoff length

We define a normalized Falk-Langer best-fit displacement gradient tensor tensor

$$\boldsymbol{F} = \underset{\boldsymbol{F}}{\mathrm{argmin}}\ \frac{1}{|\mathcal{N}_i|} \sum_{j\in\mathcal{N}_i} \frac{1}{r_{ij}(t)^{d+2}} \left|\boldsymbol{r}_{ij}(t+\Delta t) - \boldsymbol{F}\cdot\boldsymbol{r}_{ij}(t)\right|^2, \quad \mathcal{N}_i := \{j : r_{ij}(t) < \xi_{\mathrm{FL}}\}, \tag{9}$$

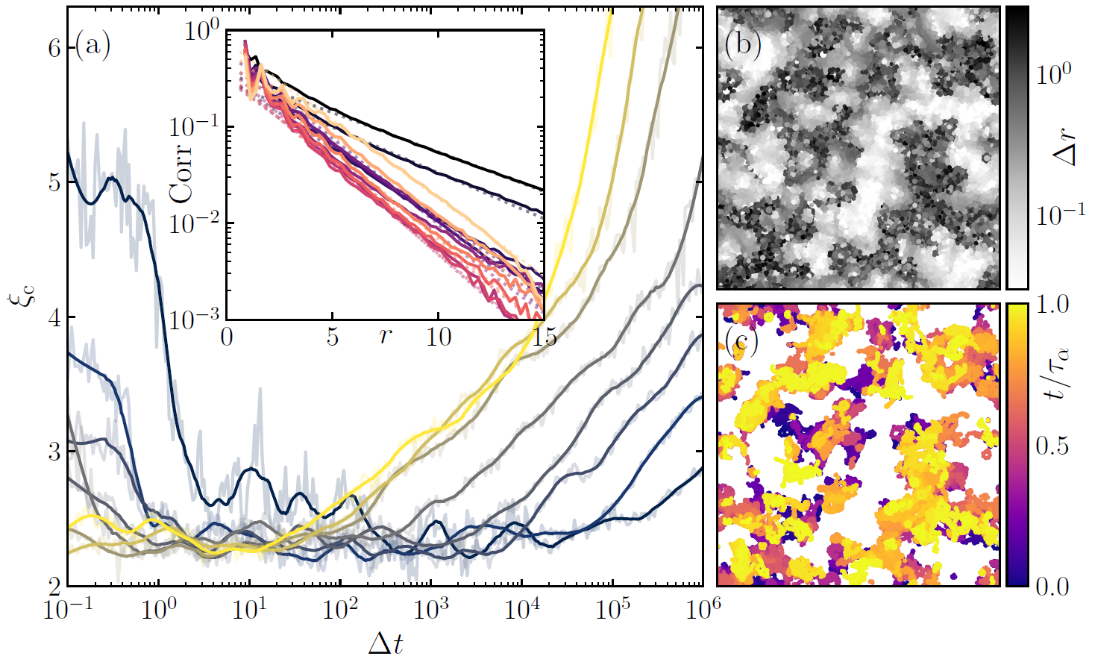


FIG. 4. *Definition of the single-rearrangement time scale, $\Delta t = 10^2$ (left) and amplitude, $\Delta_i(\Delta t) > 5$ (right).* (a): Spatial correlation length $\xi_c$ of squared particle displacement $\Delta^2$ normalized by MSD plateau height $a^2$ as a function of time interval size $\Delta t$ at temperatures $T = 0.1$, 0.12 and 0.15. The transparent curves correspond to unsmoothed data. Inset: normalized spatial correlation function for $\Delta^2/a^2$ as a function of separation $r$ at temperature $T = 0.1$ for time interval size $\Delta t = 10^{-1}$, $10^{-0.4}$, $10^{0.2}$, …, $10^{5.6}$ (curves darker to lighter). The dashed curves are fits to an exponential decay. (b): Displacement magnitude $\Delta r(0, \tau_\alpha)$ field across a time interval $\tau_\alpha$ for a system, at $T = 0.12$. (c): Positions of particles that meet the rearrangement criterion $\Delta_i > 5$ between times $t$ and $t + \Delta t$, with $\Delta t = 10^2$, for $t \in [0, \tau_\alpha]$ with values spaced $\Delta t$ apart. Color corresponds to the time of the hop, with $t$ increasing as the color gets lighter.

where $r_{ij} := |\boldsymbol{r}_{ij}|$, and $\xi_{\mathrm{FL}}$ is the radius of the neighborhood used in our strain calculation. This form is obtained from the standard form described in [9] by dividing by the number $|\mathcal{N}_i|$ of neighbors within $\xi_{\mathrm{FL}}$ (whose typical value will vary with particle diameter), dividing $\boldsymbol{r}_{ij}(t + \Delta t)$ and $\boldsymbol{r}_{ij}(t)$ by $r_{ij}$ to remove the bias towards neighbors at large separations in the standard definition, and dividing $|\boldsymbol{r}_{ij}(t + \Delta t) - \boldsymbol{F} \cdot (\boldsymbol{r}_{ij}(t))|^2$ by $r_{ij}^d$ to account for the fact that the number of neighbors in a thin shell at distance $r_{ij}$ grows as $r_{ij}^d$ in $d$ dimensions. Under this definition, we find that our results are insensitive to the specific value of $\xi_{\mathrm{FL}}$, as shown in Fig. 6. Importantly, this robustness relies on us normalizing $\boldsymbol{F}$ in the way we described, and disappears under the un-normalized definition of $\boldsymbol{F}$. We thus adopt the definition of Eq. (9) for $\boldsymbol{F}$ and set $\xi_{\mathrm{FL}} = 3$ for the results presented in the main document.

## II. TIME REVERSIBILITY

### A. Symmetries

Consider a rearranging particle $i$ with local strain tensor $\boldsymbol{E}$, and neighbouring particle $j$ a displacement $\boldsymbol{r}_{ij}$ away. In a frame reoriented such that the extensional axis local to $i$ is horizontal, $\boldsymbol{r}_{ij}$ has components $(\boldsymbol{r}_{ij} \cdot \boldsymbol{e}_{\mathrm{ext}}, \boldsymbol{r}_{ij} \cdot \boldsymbol{e}_{\mathrm{com}})$. However, the signs of the unit eigenvectors $\boldsymbol{e}_{\mathrm{ext}}$ and $\boldsymbol{e}_{\mathrm{com}}$ are arbitrary, so we can, without loss of generality, take $\boldsymbol{r}_{ij}$ to have components $(|\boldsymbol{r}_{ij} \cdot \boldsymbol{e}_{\mathrm{ext}}|, |\boldsymbol{r}_{ij} \cdot \boldsymbol{e}_{\mathrm{com}}|)$ in the reoriented frame.

The time-reversibility of our equilibrium system allows us to further simplify our analysis in certain cases. Time reversal corresponds to $\boldsymbol{E} \mapsto -\boldsymbol{E}$ and the extensional and compressional axes $\boldsymbol{e}_{\mathrm{ext}}$ and $\boldsymbol{e}_{\mathrm{com}}$ swapping directions with each other, so any time-reversible (symmetric or antisymmetric with respect to time reversal) field $f(\boldsymbol{r})$ will have to satisfy $f(|\boldsymbol{r}_{ij} \cdot \boldsymbol{e}_{\mathrm{ext}}|, |\boldsymbol{r}_{ij} \cdot \boldsymbol{e}_{\mathrm{com}}|) = \pm f(|\boldsymbol{r}_{ij} \cdot \boldsymbol{e}_{\mathrm{com}}|, |\boldsymbol{r}_{ij} \cdot \boldsymbol{e}_{\mathrm{ext}}|)$, with the sign of the RHS positive in the symmetric case and negative in the antisymmetric case.

None of the fields we look at in this report are exactly time-reversible. For instance, the strain fields are calculated based on the position $\boldsymbol{r}$ of particles relative to a rearranging particle *at the start of the rearrangement*, breaking time reversibility. Similarly, for one-time quantities, we use an Eulerian reference frame, which breaks time reversal since

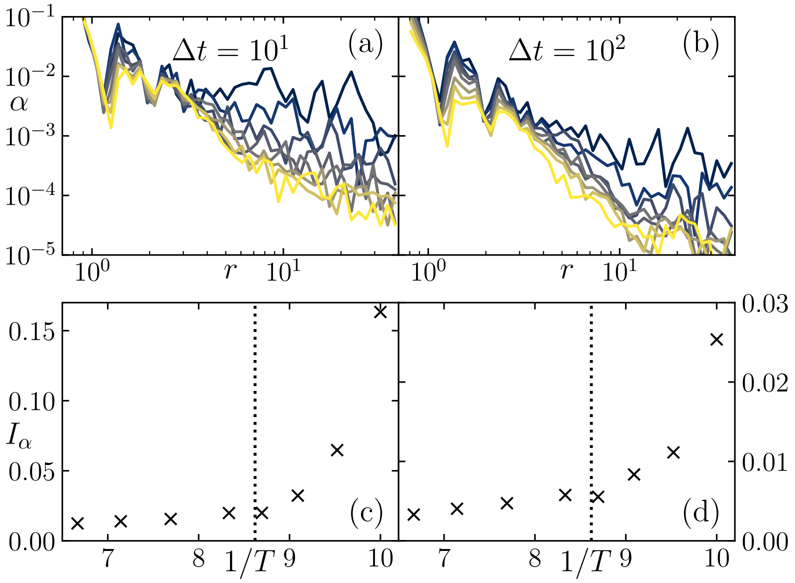


FIG. 5. *Robustness of the key result against* $\Delta t$. Plots of the mean squared anisotropy decay $\alpha(r)$ (top row) and corresponding integral $\int_{2.5}^{40} \alpha(r)\mathrm{d}r$ (bottom row) calculated over 10 trajectories for each of 202 initial equilibrium configurations for (a,c) $\Delta t = 10^1$ and (b,d) $\Delta t = 10^2$ for temperatures $T = 0.1$, 0.105, 0.11, 0.115, 0.12, 0.13, 0.14, and 0.15 (colors darker to lighter). The vertical dotted lines corresponds to $1/T_{\mathrm{MCT}}$.

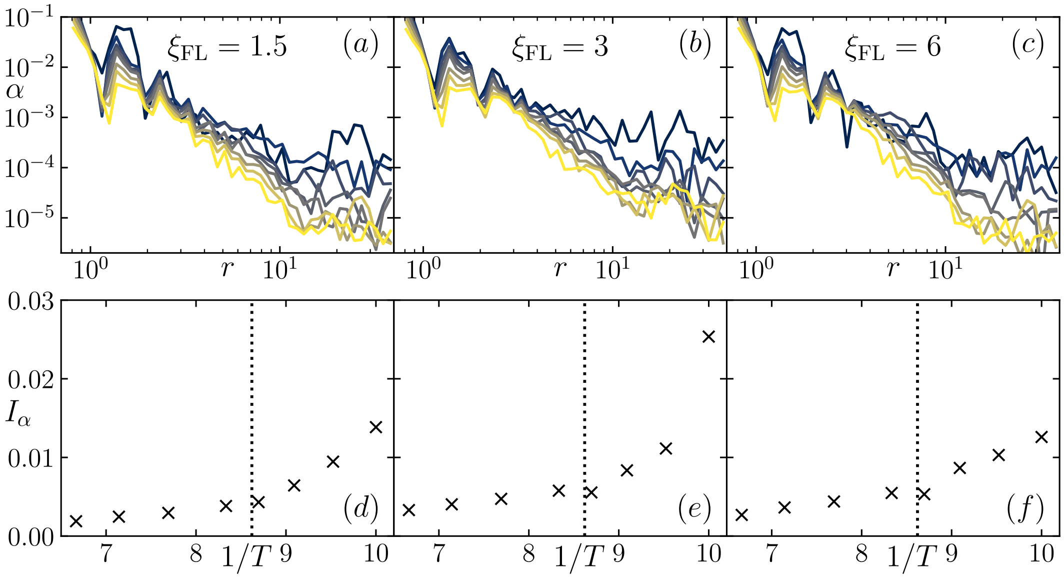


FIG. 6. *Robustness of the key result against* $\xi_{\mathrm{FL}}$. Plots of the mean squared anisotropy decay $\alpha(r)$ (top row) and corresponding integral $\int_{2.5}^{40} \alpha(r)\mathrm{d}r$ (boottom row) calculated over 10 trajectories for each of 202 initial equilibrium configurations for (a,d) $\xi_{\mathrm{FL}} = 1.5$, (b,e) $\xi_{\mathrm{FL}} = 3$, and (c,f) $\xi_{\mathrm{FL}} = 6$ for temperatures $T = 0.1$, 0.105, 0.11, 0.115, 0.12, 0.13, 0.14, and 0.15 (colors darker to lighter). The vertical dotted lines corresponds to $1/T_{\mathrm{MCT}}$.

there is a rearranging particle at the origin at the start of the interval but not at the end. In both cases, time-reversal symmetry is largely restored at larger distances, where particles are less strongly perturbed by the rearrangement and have the relative size of their displacements shrunk by their larger distance to the rearranging particle. This then explains the time-symmetric features seen at large $r$ in all polar plots in this report.

### B. Disjoint intervals

In this report, we have considered pairs of rearrangements within the same rearrangement interval $[0, \Delta t]$. Given evidence of rearrangements triggering further rearrangements, this results in ambiguity concerning the causal relationship between pairs of rearrangements. However, time reversibility means that this ambiguity is unavoidable. Even if we consider rearrangements across separate intervals $[0, \Delta t]$ and $[\Delta t, 2\Delta t]$, time reversibility still implies that there is no meaningful way to say that one rearrangement was the cause of the other, as opposed to the other way around.

Nonetheless, we plot, in Fig. 7, a comparison of the mean squared anisotropy of the pair distribution of rearrangements when using the same or disjoint intervals. We perform this comparison using a smaller rearrangement time, $\Delta t = 10^1$, as in Fig. 5.

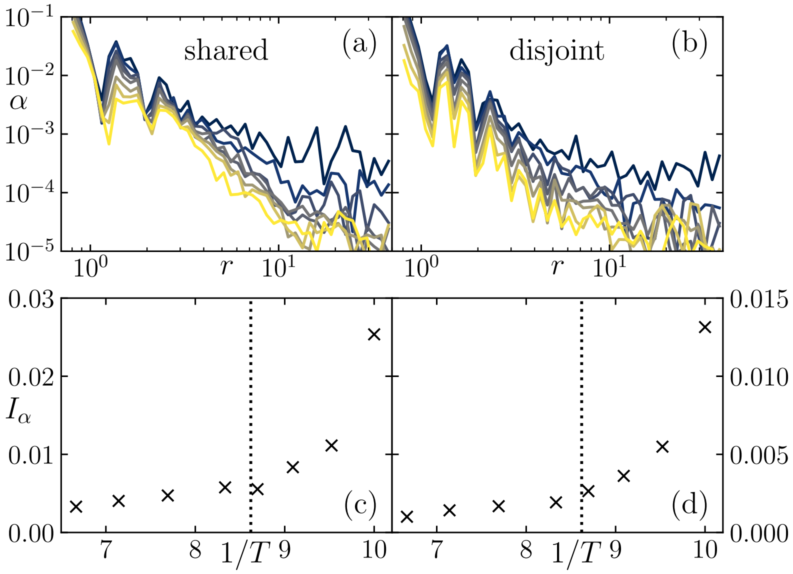


FIG. 7. *Robustness of the key result against choosing shared or disjoint time intervals.* Plots of the mean squared anisotropy decay $\alpha(r)$ (top row, c.f. main text Fig. 3(c)) and corresponding integral $\int_{2.5}^{40} \alpha(r) \mathrm{d}r$ (bottom row), calculated over 400 trajectories for each of 202 initial equilibrium configurations for (a,c) a single, or (b,d) disjoint intervals, using $\xi_{\mathrm{FL}} = 3$ and a rearrangement interval $\Delta t = 10^1$ for temperatures $T = 0.1$, 0.105, 0.11, 0.115, 0.12, 0.13, 0.14, and 0.15 (colors darker to lighter).

## III. CHARACTERIZATION OF STRAIN PERTURBATION

In the main text, we look at specific Fourier series coefficients of $\gamma_{\mathrm{iso}}$, $\gamma_{\mathrm{dev}}$, and $\gamma_{\mathrm{ext}}$ of the strain tensor $\boldsymbol{E}(\boldsymbol{r})$. With the exception of $\hat{\gamma}_{\mathrm{iso},0}$, these are the only coefficients predicted to be non-zero by continuum elasticity theory. In Fig. 8, we show that these coefficients, in addition to $\hat{\gamma}_{\mathrm{ext},0}$, are the only coefficients of magnitude greater than the noise floor of our data. Here, $\gamma_{\mathrm{flow}}$ is the off-diagonal component of $\boldsymbol{E}'$.

## IV. PAIR DISTRIBUTION OF HOPS

### A. Controlling for statistical noise

The main result of our paper concerns the pair distribution of hops

$$g_{\mathrm{hop}}(\boldsymbol{r}, t) := \frac{|\mathcal{R}|}{N} \left\langle \sum_{\substack{j \in \mathcal{R} \\ j \neq i}} \delta\left(\boldsymbol{r} - \boldsymbol{r}_{ij}(t)\right) \right\rangle_{i \in \mathcal{R}}, \tag{10}$$

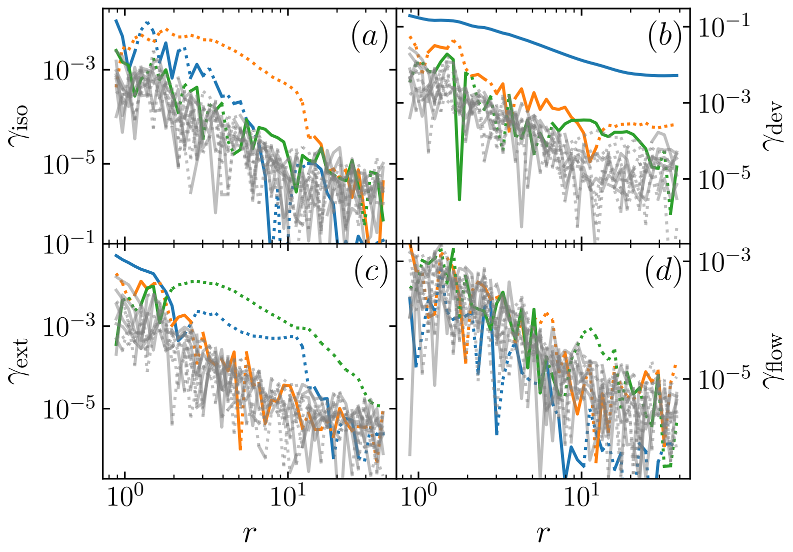


FIG. 8. *Fourier series analysis of* $\boldsymbol{E}$. (a-d): Fourier series cofficients of $\gamma_{\mathrm{iso}}$, $\gamma_{\mathrm{dev}}$, $\gamma_{\mathrm{ext}}$, and $\gamma_{\mathrm{flow}}$, respectively, as a function of distance $r$ from a rearranging particle for a system at temperature $T = 0.1$. Dotted segments denote negative values. The colors correspond to the (blue) zeroth, (orange) second, and (green) fourth Fourier modes. Fourier modes six and above are colored gray.

where $\mathcal{R}$ is the set of rearranging particles (see §I D). Specifically, we are concerned with the mean squared anisotropy $\alpha(r) = \int_0^{2\pi} \left(\tilde{g}_{\mathrm{hop}}(r,\theta) - 1\right)^2 \frac{\mathrm{d}\theta}{2\pi}$, where $\tilde{g}_{\mathrm{hop}}(r,\theta) := g_{\mathrm{hop}}(r,\theta) \,/ \int_0^{2\pi} g_{\mathrm{hop}}(r,\theta) \frac{\mathrm{d}\theta}{2\pi}$ is a normalized version of $g_{\mathrm{hop}}$, equal to 1 at a given $r$ if the distribution is perfectly isotropic, as well as its integral $I_\alpha := \int_{2.5}^{40} \alpha(r)\mathrm{d}r$. The quantity $\alpha$ is sensitive to a finite sampling effect (statistical noise). Concretely, in a situation of perfect isotropy, a finite number of samples will result in a finite (non zero) $\alpha$. The smaller the sample size, the larger the $\alpha$ measured (above the "true" $\alpha$ value corresponding to infinite sample size). Because larger temperatures have a greater number of rearrangements (more samples), they will automatically appear more isotropic. Thus, the trend observed in a naïve calculation of $\alpha$ is biased towards displaying more isotropy at higher temperatures. To control for this we calculate $\alpha$ using a modified $g_{\mathrm{hop}}$, whose underlying histogram is calculated as follows.

In the usual case, for a given set of radial and angular bins, indexed $m$ and $n$, respectively, one populates the histogram $h(m,n)$ by

1. initializing $h(m,n) = 0 \quad \forall m, n$,
2. iterating over configurations, trajectories and rearrangements, and
3. for each rearrangement $i$, updating $h(m,n) \mapsto h(m,n) + h_i(m,n)$, where $h_i$ is the histogram of the positions of the other rearrangements $j \neq i$ relative to rearrangement $i$.

When calculating the modified $g_{\mathrm{hop}}$, we first compute $h(m,n)$ in the naïve way for our coldest temperature $T = 0.1$, and denote it for future reference as $h_*(m,n)$. Its angular-integrated value $H_*(m) = \sum_n h_*(m,n)$ represents the number of samples available in the radial distance bin $m$, for the temperature $(T = 0.1)$ at which we have the least samples. For all other temperatures, we replace the third step with

3. for each rearrangement $i$ and radial bin $m$, compute $h_i$, the histogram of the positions of the other rearrangements $j \neq i$ relative to rearrangement $i$, and $H_i(m) = \sum\limits_n h_i(m,n)$.
4. Compute the current $H(m) = \sum\limits_n h(m,n)$.
5. Then, for each radial bin $m$, update $h(m,n) \mapsto h(m,n) + h_i(m,n)$ only if $|H(m) + H_i(m) - H_*(m)| \leq |H(m) - H_*(m)|$. That is to say, update element $(m,n)$ of the histogram $h$ with the available samples counted in $h_i(m,n)$ only if doing so for a given $m$ and all angular bins $n$ will bring $H(m) = \sum\limits_n h(m,n)$ closer to $H_*(m) = \sum\limits_n h_*(m,n)$, recalling that $h_*$ is the naïve histogram for the temperature $(T = 0.1)$ at which we have the least samples.

This procedure results in an almost perfect match between the number of samples per radial bin for each temperature (across all temperatures $T$ and radial bins $m$, the maximum relative difference between the populations of radial bin $m$ at temperature $T$ and at temperature 0.1 is $2 \times 10^{-5}$), and eliminates the possibility that the trend seen in $\alpha$ as a function of $T$ is simply due to having better statistics at higher $T$.

### B. Lower limit of integration

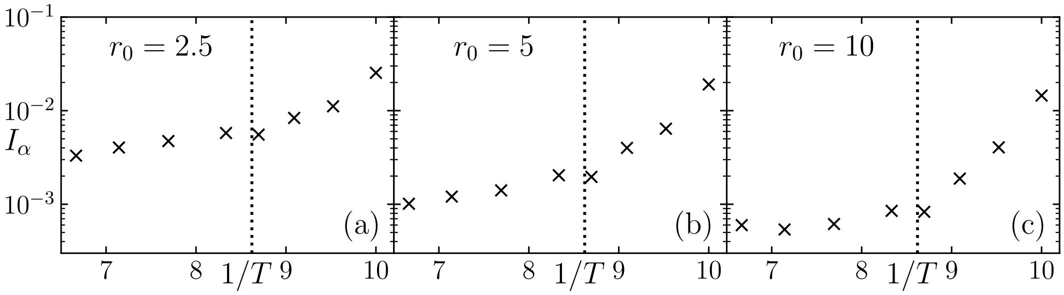


FIG. 9. *Robustness of the key result against the choice of* $r_0$. Plots of the mean squared anisotropy integral $I_\alpha = \int_{r_0}^{40} \alpha(r)\mathrm{d}r$ calculated over 10 trajectories for each of 202 initial equilibrium configurations for lower bounds (a) $r_0 = 2.5$, (b) $r_0 = 5$, and (c) $r_0 = 10$ as a function of reciprocal temperature. The vertical dotted lines corresponds to $1/T_{\mathrm{MCT}}$.

In the main text, we noted an apparent crossover at $T = T_{\mathrm{MCT}}$ when $\alpha(r)$ is integrated between the end of the second neighbor shell $r_0 = 2.5$ and $r_\infty = 40$, above which finite size effects due to our periodic boundary conditions become apparent. Here, we show that the existence and location of this crossover in $I_\alpha$ is robust to varying the lower bound $r_0 = 2.5$. In Fig. 9, we see a kink, or at least inflection point, at $T = T_{\mathrm{MCT}}$ for three lower bounds $r_0 \in \{2.5, 5, 10\}$ in the definition of $I_\alpha$, $I_\alpha = \int_{r_0}^{40} \alpha \mathrm{d}r$. Here, contrary to the presentation of the main text, $I_\alpha$ is presented in log scale to ease the comparison between $r_0$ values, which also makes the crossover less visually dramatic. One should note that for each choice of $r_0$, $\alpha(r)$ spans at most 1.5 orders of magnitude, justifying the choice of linear scale in the main text.

### C. Number density of rearrangements

In the main text, we discuss how signals in the elastic response to a plastic rearrangement event may be obscured by the presence of other rearrangements, and that this will happen at increasingly small distances from the plastic event as $T$ increases. To illustrate this, we plot in Fig. 10(a) the density $\rho_{\mathrm{hop}}$ of rearrangements across a time interval $\Delta t = 10^2$. From $\rho_{\mathrm{hop}}$, assuming a uniform hop distribution, we can obtain the estimate $r_{\mathrm{hop}} = \Gamma(3/2)/\sqrt{\pi \rho_{\mathrm{hop}}}$. This estimate is computed as the mean closest distance between two points in $\mathbb{R}^2$ in a uniformly distributed set of points at number density $\rho_{\mathrm{hop}}$ [10], *i.e.* as the typical distance between nearest neighbour rearrangements under the hypthesis of uniform event occurence. We plot $r_{\mathrm{hop}}$ in Fig. 10(b). We see that $\rho_{\mathrm{hop}}$ decreases rapidly as an expontial function of $1/T$, resulting in an order-of-magnitude increase in $r_{\mathrm{hop}}$ between our highest temperature, $T = 0.150$, and our lowest, $T = 0.100$. This suggests a rapid increase in the typical distance between uncorrelated rearrangements with decreasing temperature.

### D. Multipolarity of the pair distribution function

We further characterize the anisotropic nature of the pair distribution of rearrangements via the Fourier series expansion of $\tilde{g}_{\mathrm{hop}}$. As shown in Fig. 11, the only Fourier modes $\hat{\tilde{g}}_{\mathrm{hop},k}$ that rise above the noise floor, other than the zeroth mode $\hat{\tilde{g}}_{\mathrm{hop},0} \equiv 1$, are the dipolar and quadrupolar terms $\hat{\tilde{g}}_{\mathrm{hop},2}$ and $\hat{\tilde{g}}_{\mathrm{hop},4}$. The dipolar term has only a slight increase in magnitude with decreasing temperature $T$, whereas at intermediate-to-large distances $r \gtrsim 5$, the difference in size of $\hat{\tilde{g}}_{\mathrm{hop},4}$ between the highest and lowest temperatures grows to two orders of magnitude.

This behaviour highlights the long-ranged character of the elastoplastic mechanism for correlating rearrangements: the anisotropy is preserved, even up to distances at which time reversal symmetry is unbroken. As discussed in §II A,

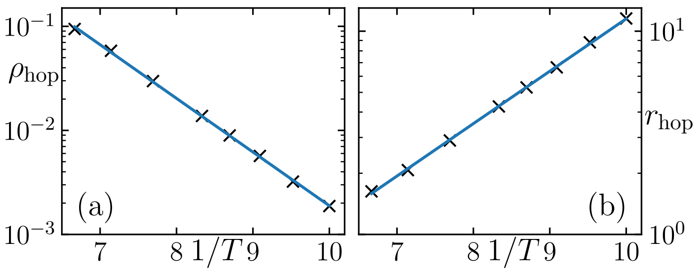


FIG. 10. *Distance between hops.* Plots of (a) the number density $\rho_{\rm hop}$ of rearrangements across the rearrangement time interval $\Delta t = 10^2$ and (b) the corresponding mean minimum distance $r_{\rm hop}$ between rearrangements for a uniform distribution of rearrangements at number density $\rho_{\rm hop}$ as a function of inverse temperature $1/T$. Blue line: exponential fits (a) $A \exp\left(-\frac{T_*}{T}\right)$ and (b) $\frac{1}{\sqrt{\pi A}}\Gamma\left(\frac{3}{2}\right)\exp\left(\frac{T_*}{2T}\right)$ to the data, where $A = 272$ and $T_* = 1.188$.

our definition of $g_{\rm hop}$, in terms of the relative positions of rearrangements at the start of a rearrangement interval, breaks time reversal symmetry at short distances, but not at large distances. Time reversibility implies symmetry under exchange of extensional and compressional axes, so the dipolar term, which violates this symmetry, must vanish at distances at which time reversal symmetry is preserved.

Physical insight into the mechanisms underlying this behaviour is provided by reference to Figs. 1 and 2 of the main text. The deviatoric strain, $\gamma_{\rm dev}$, is isotropic, so the isotropic strain $\gamma_{\rm iso}$ provides the only source of rotational symmetry breaking. However, $\gamma_{\rm iso}$ is at best an order of magnitude smaller than $\gamma_{\rm dev}$, increasing to two orders of magnitude for the highest temperature $T = 0.15$. This dominance of the isotropic $\gamma_{\rm dev}$ explains why anisotropy in $\tilde{g}_{\rm hop}$ is so subtle, while the trend in the relative sizes of $\gamma_{\rm dev}$ and $\gamma_{\rm iso}$ with temperature explains the increasing anisotropy with decreasing $T$ that we observe. Furthermore, we see that $\gamma_{\rm iso}$ is negative along the extensional axis, so that the preference for rearrangements along this direction seen in Fig. 11(e), corresponds to an increased propensity to rearrangement where the plastic event has caused particles to move closer to one another, increasing the local potential energy. Finally, the increasingly strong constraint of time reversibility with increasing $r$, applied to a dipolar signal, explains the dominance of $\hat{\tilde{g}}_{\rm hop,2}$ at small separations, and the eventual dominance of the $\hat{\tilde{g}}_{\rm hop,4}$ term over the $\hat{\tilde{g}}_{\rm hop,2}$ term at large separations.

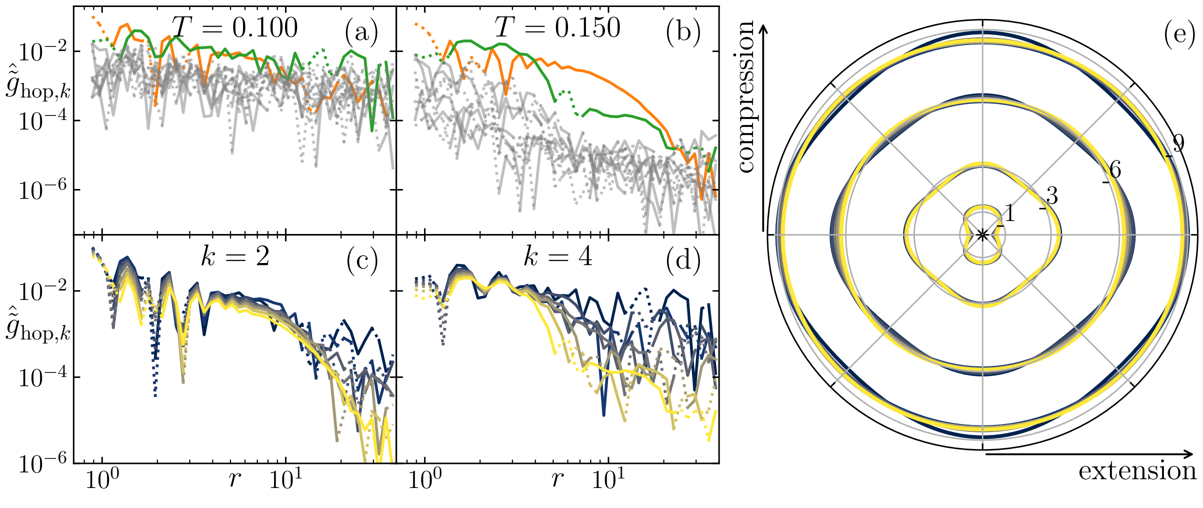


FIG. 11. *Fourier modes of* $\tilde{g}_{\rm hop}$. Top row: Fourier series expansion coefficients of $\tilde{g}_{\rm hop}$ at temperatures (a) $T = 0.105$ and (b) 0.150. The $k = 2$ mode is shown in orange, the $k = 4$ mode in green, and modes $k > 4$ are shown in gray, as an estimate of the height of the noise floor. The $k = 0$ mode $\hat{\tilde{g}}_{\rm hop,0} \equiv 1$ by definition, and is not shown here. Bottom row: Fourier modes (c) $k = 2$ and (d) $k = 4$ at temperatures $T = 0.100$, 0.105, 0.110, 0.115, 0.120, 0.130, 0.140, and 0.150 (curves darker to lighter; dotted segments denote negative values). Polar plot: Fourier series expansion of $\tilde{g}_{\rm hop}$ truncated at fourth-order, at radii $r = 1$, 3, 6, 9, scaled such that isotropy of $\tilde{g}_{\rm hop}$ at a given $r$ value corresponds to a circle of radius $r$. The curves correspond to different temperatures, colored as per (c) and (d).

[1] E. Flenner and G. Szamel, Nat. Commun. **6**, 7392 (2015).
[2] S. Vivek, C. P. Kelleher, P. M. Chaikin, and E. R. Weeks, Proc. Natl. Acad. Sci. U.S.A. **114**, 1850 (2017).
[3] B. Illing, S. Fritschi, H. Kaiser, C. L. Klix, G. Maret, and P. Keim, Proc. Natl. Acad. Sci. U.S.A. **114**, 1856 (2017).
[4] R. Das, I. Tah, and S. Karmakar, J. Chem. Phys. **149**, 024501 (2018).
[5] N. Lačević, F. W. Starr, T. B. Schrøder, and S. C. Glotzer, J. Chem. Phys. **119**, 7372 (2003).
[6] I. Tah, S. Sengupta, S. Sastry, C. Dasgupta, and S. Karmakar, Phys. Rev. Lett. **121**, 085703 (2018).
[7] L. Berthier, P. Charbonneau, A. Ninarello, M. Ozawa, and S. Yaida, Nat. Commun. **10**, 1508 (2019).
[8] E. D. Cubuk, R. J. S. Ivancic, S. S. Schoenholz, D. J. Strickland, A. Basu, Z. S. Davidson, J. Fontaine, J. L. Hor, Y.-R. Huang, Y. Jiang, N. C. Keim, K. D. Koshigan, J. A. Lefever, T. Liu, X.-G. Ma, D. J. Magagnosc, E. Morrow, C. P. Ortiz, J. M. Rieser, A. Shavit, T. Still, Y. Xu, Y. Zhang, K. N. Nordstrom, P. E. Arratia, R. W. Carpick, D. J. Durian, Z. Fakhraai, D. J. Jerolmack, D. Lee, J. Li, R. Riggleman, K. T. Turner, A. G. Yodh, D. S. Gianola, and A. J. Liu, Science **358**, 1033 (2017).
[9] M. L. Falk and J. S. Langer, Phys. Rev. E **57**, 7192 (1998).
[10] S. Chandrasekhar, Rev. Mod. Phys. **15**, 1 (1943).
